# Supplementary material for: f-GANs in an Information Geometric Nutshell
Source: arXiv:1707.04385 source file (2017-07-14)
Supplement: Supplementary file 1 [file arxiv-gan-proof-viggan.tex]

\newpage
%Why limit above ? if P = 0 ?

%f continuous, $f(1) << infty$, defined on [0, a), a eventually +infty

Let $\mathbb{I}_{P,Q} \defeq [\inf_{\ve{x}} P(\ve{x})/Q(\ve{x}),
\sup_{\ve{x}} P(\ve{x})/Q(\ve{x}))$.
\begin{theorem}\label{thVIGGEN1}
Suppose $f$ convex and continuous. For any densities $P$, $Q$, if
$\exists \xi \in \partial f$ such that $\sup \xi(\mathbb{I}_{P,Q}) <
\infty$, then $\exists
\chi : \mathbb{R}_+ \rightarrow \mathbb{R}_+$ increasing such that $I_f(P\|Q) = KL_\chi(Q\|P)$.
\end{theorem}
Suppose there exists $M \in \mathbb{R}$ such that
$\sup \xi(\mathbb{I}_{P,Q}) \leq M$, for some $\partial f \ni \xi : \mbox{ int }\mathrm{dom}(f) \rightarrow
\mathbb{R}$.
For any constants $k$, letting $f_{k}(z) \defeq
f(z) - k(z-1)$, which is convex and continuous since $f$ is, we
note that
\begin{eqnarray}
\expect_{\X\sim
  Q}\left[f_{k}
  \left(\frac{P(\X)}{Q(\X)}\right)\right] & = & \expect_{\X\sim
  Q}\left[f
  \left(\frac{P(\X)}{Q(\X)}\right)\right] - k\cdot \expect_{\X\sim
  Q}\left[\frac{P(\X)}{Q(\X)} - 1\right]\nonumber\\
 & = &  \expect_{\X\sim
  Q}\left[f
  \left(\frac{P(\X)}{Q(\X)}\right)\right] - k\cdot \left(\int P(\X)
\mathrm{d}\mu(\X) - \int Q(\X)
\mathrm{d}\mu(\X)\right)\nonumber\\
 & = & \expect_{\X\sim
  Q}\left[f
  \left(\frac{P(\X)}{Q(\X)}\right)\right]\:\:.\label{inv1}
\end{eqnarray}
Let $\xi_k \defeq \xi - k \in \partial f_{k}$.
Since $f_k$ is convex continuous, it follows from \cite[Proposition
1.6.1]{npCF} that:
\begin{eqnarray}
f_k\left(\frac{P(\ve{x})}{Q(\ve{x})}\right) & = & f_{k}(1)
+ \lim_{\rho \rightarrow \frac{P(\ve{x})}{Q(\ve{x})}} \int_{1}^{\rho}
\xi_{k}(t) \mathrm{d}t\nonumber\\
& = &  -\lim_{\rho \rightarrow \frac{P(\ve{x})}{Q(\ve{x})}} \int_{1}^{\rho}
(-\xi(t)+k) \mathrm{d}t\:\:. \label{inv2}
\end{eqnarray}
The second identity comes from the assumption that $f(1) = 0 = f_{k}(1)$.
The limit does not appear in the statement of \cite[Proposition
1.6.1]{npCF}, we make it appear to cope with a subdifferential that would not
be Riemann integrable. Fix some constant $\epsilon > 0$ and let
\begin{eqnarray}
\chi (t) & = & \left\{
\begin{array}{rcl}
\frac{1}{-\xi(t) + M +\epsilon} & \mbox{ if } & t < \sup_{\ve{x}} P(\ve{x})/Q(\ve{x})\:\:,\\
\frac{1}{\epsilon} & \mbox{ if } & t \geq \sup_{\ve{x}} P(\ve{x})/Q(\ve{x})
\end{array}
\right.\:\:,\label{defchi1}
\end{eqnarray}
which, since $\sup \xi (\mathbb{I}_{P,Q}) \leq M$, guarantees $\chi \geq 0$ and $\chi$ is also increasing
since $\xi$ is increasing ($f$ is convex). We then check, using
eqs. (\ref{inv1}) and (\ref{defchi1}) that:
\begin{eqnarray}
KL_\chi(Q\|P) & = & \expect_{\X\sim
  Q}\left[-\log_\chi
  \left(\frac{P(\X)}{Q(\X)}\right)\right] \nonumber\\
 & = & \expect_{\X\sim
  Q}\left[-\lim_{\rho \rightarrow \frac{P(\X)}{Q(\X)}} \int_{1}^{\rho}
\frac{1}{\chi(t)} \mathrm{d}t \right] \nonumber\\
 & = & \expect_{\X\sim
  Q}\left[-\lim_{\rho \rightarrow \frac{P(\X)}{Q(\X)}} \int_{1}^{\rho}
(-\xi(t) + M +\epsilon) \mathrm{d}t \right] \nonumber\\
 & = & \expect_{\X\sim
  Q}\left[f_{M+\epsilon}
  \left(\frac{P(\X)}{Q(\X)}\right) \right] \nonumber\\
 & = & \expect_{\X\sim
  Q}\left[f
  \left(\frac{P(\X)}{Q(\X)}\right) \right] = I_f(P\|Q) \:\:.
\end{eqnarray}
\begin{corollary}\label{corGEN}
Suppose $f$ convex, continuous and such that $\exists \xi \in \partial
f$ with $\sup \xi(\mathrm{int } \mathrm{dom} f) <
\infty$. Then $\exists
\chi : \mathbb{R}_+ \rightarrow \mathbb{R}_+$ increasing such that
for any densities $P$, $Q$, $I_f(P\|Q) = KL_\chi(Q\|P)$.
\end{corollary}
In Corollary \ref{corGEN}, $\chi$ does not depend on $P$ and $Q$. In
Theorems \ref{thVIGGEN1} and \ref{thVIGGEN2}, it does depend on $P$
and $Q$, but does not change as a function of $\ve{x}$. In the GAN
game, it makes sense to assume $I_f<\infty$ since otherwise the
solution is vacuous (ref to eq).

\newpage

\begin{theorem}\label{thVIGGEN2}
Suppose $f$ convex and continuous. For any densities $P$, $Q$, if
$\sup \xi(\mathbb{I}_{P,Q}) = +\infty, \forall \xi \in \partial f$, but 
$I_f(P\|Q) < +\infty$, then $\forall \delta
> 0$, $\exists
\chi : \mathbb{R}_+ \rightarrow \mathbb{R}_+$ increasing such that
\begin{eqnarray}
KL_\chi(Q\|P) \leq I_f(P\|Q) \leq KL_\chi(Q\|P) + \delta\:\:.
\end{eqnarray}
\end{theorem}
Without loss of generality we can assume that $\sup \mathbb{I}_{P,Q} <
+\infty$. Otherwise, when $\sup \mathbb{I}_{P,Q} = + \infty$,
requesting $\sup \xi(\mathbb{I}_{P,Q}) = +\infty$ ($\forall \xi \in \partial
f$) implies, because $f$
is convex continuous, that $\lim_{\sup
  \mathbb{I}_{P,Q}}f(z) = +\infty$, and so the constraint $I_f(P\|Q) <
+\infty$ essentially enforces zero measure over all infinite density ratios.

We make use of \cite[Proposition 1.6.1]{npCF}, now with a
subdifferential which is not Riemann integrable in $M \defeq \sup
\mathbb{I}_{P,Q}$. Notice that we can assume without loss of
generality that $M > 1$ since otherwise, since it is convex and
continuous, $f$ would not be defined for $z> 1$ and $I_f(P\|Q)$
would essentially be infinite unless $Q \geq P$ almost everywhere
(\textit{i.e.} $P$ dominates $Q$ only on sets of zero measure).\\

For any constants
$t^* < M, \epsilon$ such that $\xi(t^*) < +\infty$, let
\begin{eqnarray}
g_{t^*,\epsilon}(z) & \defeq & \int_{1}^{z}
(-\xi(t)+\xi(t^*)+\epsilon)\mathrm{d}t\:\:, 
\end{eqnarray}
where $z \in \mathbb{R}_+$ is any real such that the integral in
$g_{t^*,\epsilon}$ is not improper
(therefore, $z< M$). Let
\begin{eqnarray}
\chi_{t^*,\epsilon}(t) & = & \left\{
\begin{array}{rcl}
\frac{1}{-\xi(t) +\xi(t^*)+\epsilon} & \mbox{ if } & t < t^*\:\:,\\
\frac{1}{\epsilon} & \mbox{ if } & t \geq t^*
\end{array}
\right.\:\:,
\end{eqnarray}
which, if $\epsilon > 0$, is non negative and also increasing
since $\xi $ is increasing. Consider any fixed $z^* \in \mathbb{I}_{P,Q}
\cap (1,\infty)$ with $0<\xi(z^*) < \infty$ and let $t^* \defeq \sup
\{z : \xi(z) \leq \xi(z^*)\}$. We have:
\begin{eqnarray}
g_{t^*,\epsilon}(z) & = & \int_{1}^{z}
(-\xi(t)+\xi(t^*)+\epsilon)\mathrm{d}t\nonumber\\
& = & \int_{1}^{z}
\frac{1}{\chi_{t^*,\epsilon}(t)} \mathrm{d}t + 1_{[z \geq t^*]} \cdot \int_{t^*}^{z}
(-\xi(t)+ \xi(t^*))\mathrm{d}t\nonumber\\
& =  & \int_{1}^{z}
\frac{1}{\chi_{t^*,\epsilon}(t)} \mathrm{d}t  -
1_{[z \geq t^*]} \cdot \int_{t^*}^{z}
(\xi(t)- \xi(t^*))\mathrm{d}t\nonumber\\
 & = & \int_{1}^{z}
\frac{1}{\chi_{t^*,\epsilon}(t)} \mathrm{d}t  -
1_{[z\geq t^*]} \cdot D_{f,
  \xi}\left(\left. z\right\| t^*\right) \label{inv3}\:\:.
\end{eqnarray}
The last identity comes from \cite[Proposition 1.6.1]{npCF} and the
fact that $\xi(t)- \xi(t^*)$ belongs to the subdifferential of the
Bregman divergence whose generator is $f$ \cite{frCF}. We obtain:
\begin{eqnarray}
\lefteqn{\expect_{\X\sim
  Q}\left[f
  \left(\frac{P(\X)}{Q(\X)}\right)\right]}\nonumber\\
 & = & \expect_{\X\sim
  Q}\left[f_{\xi(t^*)+\epsilon}
  \left(\frac{P(\X)}{Q(\X)}\right)\right]\label{cons11}\\
 & = & \expect_{\X\sim
  Q}\left[\lim_{\rho \rightarrow \frac{P(\X)}{Q(\X)}} -\int_{1}^{\rho}
(-\xi(t)+\xi(t^*)+\epsilon) \mathrm{d}t\right]\label{cons12}\\
 & = & \expect_{\X\sim
  Q}\left[\lim_{\rho \rightarrow \frac{P(\X)}{Q(\X)}} -g_{t^*,\epsilon}(\rho)\right]\nonumber\\
 & = & \expect_{\X\sim
  Q}\left[\lim_{\rho \rightarrow \frac{P(\X)}{Q(\X)}}
  \left\{-\int_{1}^{\rho}
\frac{1}{\chi_{t^*,\epsilon}(t)} \mathrm{d}t +
1_{\left[\rho\geq t^*\right]} \cdot D_{f,
  \xi}\left(\left. \rho \right\| t^*\right) \right\}\right]\label{cons13}\\
 & = & \expect_{\X\sim
  Q}\left[-\lim_{\rho \rightarrow \frac{P(\X)}{Q(\X)}}
  \int_{1}^{\rho}
\frac{1}{\chi_{t^*,\epsilon}(t)} \mathrm{d}t\right] + \underbrace{\expect_{\X\sim
  Q}\left[\lim_{\rho \rightarrow \frac{P(\X)}{Q(\X)}}
1_{\left[\rho\geq t^*\right]} \cdot D_{f,
  \xi}\left(\left. \rho \right\| t^*\right) \right]}_{\defeq R(t^*)}\label{cons15}\\
 & = & \expect_{\X\sim
  Q}\left[-\log_{\chi_{t^*,\epsilon}}\left(\frac{P(\X)}{
      Q(\X)}\right)\right] + R(t^*)\label{cons16}\\
 & = & KL_{\chi_{t^*,\epsilon}}(Q\|P) + R(t^*)\label{cons17}\:\:.
\end{eqnarray}
Eq. (\ref{cons11}) follows from Eq. (\ref{inv1}).
Eq. (\ref{cons12}) follows from Eq. (\ref{inv2}).
Eq. (\ref{cons13}) follows from Eq. (\ref{inv3}). We can split the
limits in eq. (\ref{cons15}) because each term in the expectation of
$R(t^*)$ is finite. To see it, since $I_f(P\|Q) < \infty$ and $\sup
\xi (\mathbb{I}_{P,Q}) = +\infty$, we can assume that $f(M) <
+\infty$. Since $\xi(t^*) \geq
0$, then
\begin{eqnarray}
\rho \geq t^* & \Rightarrow & D_{f,
  \xi}\left(\left. \rho \right\| t^*\right) \leq f(M) - f(t^*) \:\:,
\end{eqnarray}
which is indeed finite. It then comes 
\begin{eqnarray}
\expect_{\X\sim
  Q}\left[\lim_{\rho \rightarrow \frac{P(\X)}{Q(\X)}}
1_{\left[\rho\geq t^*\right]} \cdot D_{f,
  \xi}\left(\left. \rho \right\| t^*\right) \right] & = & \expect_{\X\sim
  Q}\left[
1_{\left[\frac{P(\X)}{Q(\X)}\geq t^*\right]} \cdot D_{f,
  \xi}\left(\left. \frac{P(\X)}{Q(\X)} \right\| t^*\right)
\right]\nonumber\\
 & \leq & \expect_{\X\sim
  Q}\left[D_{f,
  \xi}(M\|t^*)
\right] \nonumber\\
 & \leq & f(M) - f(t^*)\:\:.
\end{eqnarray}
Since $f$ is continuous, we get the upperbound on $I_f(P\|Q)$ by choosing $t^*<M$ as
close as desired to $M$. We get the lowerbound by remarking that
$R(t^*) \geq 0$ (a Bregman divergence cannot be negative).

\newpage

\begin{theorem}
Letting
$P\defeq P_{\chi, C}$ and $Q \defeq Q_{\chi, C}$ for short, the following holds:
\begin{eqnarray}
\expect_{\X\sim \tilde{Q}}[\log_\chi(Q(\X)) - \log_\chi(P(\X))] & = &
KL_{\chi_{\tilde{{Q}}}}(\tilde{Q}\|P) - J(Q)\:\:,
\end{eqnarray} 
with $J(Q) \defeq
KL_{\chi_{\tilde{{Q}}}}(\tilde{Q}\|Q)$ and $\chi_{\tilde{Q}(\ve{x})}(t) \defeq (1/\tilde{Q}(\ve{x}))\cdot \chi
(t \tilde{Q}(\ve{x}))$.
\end{theorem}
The normalization $Z$ for the escort of $Q$ being
finite, it implies the finiteness of $\tilde{Q}$ almost everywhere

We have
\begin{eqnarray*}
\expect_{\tilde{{Q}}}[-(\log_\chi({P})-\log_\chi({Q}))]
& = &
\expect_{\tilde{{Q}}}[-(\log_\chi({P})-\log_\chi(\tilde{{Q}}))]
+ \expect_{\tilde{{Q}}}[-(\log_\chi(\tilde{{Q}})-\log_\chi({Q}))]\:\:.
\end{eqnarray*}
Also, 
\begin{eqnarray}
(\log_\chi({P})-\log_\chi({\tilde{{Q}}})) & = & \int_{{{1}}}^P
\frac{1}{\chi(t)} \cdot \mathrm{d}t - \int_1^{\tilde{{Q}}}
\frac{1}{\chi(t)} \cdot \mathrm{d}t\nonumber\\
& = & \int_{\tilde{{Q}}}^P
\frac{1}{\chi(t)} \cdot \mathrm{d}t\nonumber\\
 & = & \int_{1}^{\frac{P}{\tilde{{Q}}}}
\frac{\tilde{{Q}}}{\chi(t \tilde{{Q}})} \cdot \mathrm{d}t\nonumber\\
 & = & \int_{1}^{\frac{P}{\tilde{{Q}}}}
\frac{1}{\chi_{\tilde{{Q}}}(t)} \cdot \mathrm{d}t\nonumber\\
 & = & \log_{\chi_{\tilde{{Q}}}}\left(\frac{P}{\tilde{{Q}}}\right)\:\:,
\end{eqnarray}
with 
\begin{eqnarray}
\chi_{\tilde{{Q}}(\ve{x})}(t) & \defeq & \frac{1}{\tilde{{Q}} (\ve{x})}\cdot \chi
(t\tilde{{Q}}(\ve{x}))\label{defCHITILDE} 
\end{eqnarray}
satisfying $\mathrm{d} \chi_{\tilde{{Q}} (\ve{x})} /
\mathrm{d} t = \chi'
(t \tilde{{Q}} (\ve{x}))$ and so is increasing, plus $\chi_{\tilde{{Q}}}$ is
positive iff $\chi$ is positive since $\tilde{{Q}}(\ve{x})\geq 0$, so $\chi_{\tilde{{Q}}}(t)$
defines a
$\chi$-logarithm, also differentiable. Hence,
\begin{eqnarray}
\expect_{\tilde{{Q}}}[-(\log_\chi({P})-\log_\chi(\tilde{{Q}}))] & = & KL_{\chi_{\tilde{{Q}}}}(\tilde{Q}\|P)\:\:,
\end{eqnarray}
and
\begin{eqnarray}
\expect_{\tilde{{Q}}}[-(\log_\chi({Q}) - \log_\chi(\tilde{{Q}}))] & = & KL_{\chi_{\tilde{{Q}}}}(\tilde{Q}\|Q)\:\:.
\end{eqnarray}
This ends the proof of point (ii).\\

\newpage

\noindent We prove point (i). We first remark that we have $(-\log_{\chi})'' = \chi' / \chi^2 \geq 0$ and so $-\log_{\chi}$ is convex and $KL_{\chi}(P\|Q)$ is an
$f$-divergence with $f$ twice differentiable. We also notice that
$\mathrm{dom}(-\log_{\chi}) \supseteq \mathbb{R}_+$.
To show the equivalence, we extract $\chi$ from any
twice differentiable $f$-divergence and show that for this couple $(f,
\chi)$,
$KL_{\chi}(P\|Q) = I_f(P\|Q), \forall P, Q$. Let $f_\diamond(z)
\defeq z \cdot f(1/z)$ denote the Csisz\'ar dual of $f$, which is
also convex (indeed, $f''_\diamond(z) = (1/z^2)\cdot f''(z)$) and
satisfies $I_f(P\|Q) = I_{f_\diamond}(Q\|P)$. Hence, we want to prove
\begin{eqnarray}
\expect_{\X\sim P}\left[-\log_{\chi}\left(\frac{Q(\X)}{P(\X)}\right)\right] & = & \expect_{\X\sim P}
\left[f_\diamond \left(\frac{Q(\X)}{P(\X)}\right)\right]\:\:, \forall
P, Q\:\:.
\end{eqnarray}
We want 
\begin{eqnarray}
\frac{\chi'}{\chi^2} & = & f''_\diamond\:\:,
\end{eqnarray}
whose solution is easily found to be solution to the following
differential equation: $\mathrm{d}\left(-1/\chi(z)\right) = f''_\diamond(z)
\mathrm{d} z$, that is, $-1/\chi(z) = f'_\diamond(z) + k$ for any constant $k$
and therefore
\begin{eqnarray}
\chi(z) & = & -\frac{1}{f'_\diamond(z) + k}\:\:,\label{eqchif}
\end{eqnarray}
Clearly, $\chi$ is increasing since $f_\diamond$ is convex and
\begin{eqnarray}
\chi'(z) & = & \frac{f''_\diamond(z)}{(f'_\diamond(z) + k)^2}\:\:.
\end{eqnarray}
 We now
constrain the choice of $k$ to the fact that we also want $\chi(z)\geq
0$, that is, we want $k$ such that 
\begin{eqnarray}
f'_\diamond(z) & \leq & -k\:\:, \forall z\in \mathbb{R}_+\:\:.\label{constK}
\end{eqnarray}
To prove that this is indeed possible, we first remark
that for any constant $k_2\geq 0$, 
\begin{eqnarray}
f'(t) & \leq & f'(t) + t f''(t) + k_2 \:\:,\forall t\geq 0\:\:.\label{eqCONV1}
\end{eqnarray}
This is indeed obvious since $f$ is convex, and it brings after
integration between any constant $c \in \mathrm{dom} f'$ and $z$,
$f(z) - f(c) \leq z f'(z) - c f'(c) + k_2 (z-c)$, which
brings after the change of variable $z\mapsto 1/z$ and reordering:
\begin{eqnarray}
\underbrace{f\left(\frac{1}{z}\right) - \frac{1}{z} \cdot
f'\left(\frac{1}{z}\right)}_{= f'_\diamond(z)} & \leq & \frac{k_2}{z} + f(c) - cf'(c) - ck_2 \:\:,
\end{eqnarray}
so we get that we can pick $k_2=0$ which, to guarantee ineq. (\ref{constK}), yields \textit{e.g.} the choice
\begin{eqnarray}
k & = & -(f(c) - cf'(c)) = - f'_\diamond(1/c)\:\:, \label{eqKA}
\end{eqnarray}
with $c \in \mathrm{dom} f'$. For the
expression of $\chi$ in (\ref{eqchif}), we obtain 
\begin{eqnarray}
-\log_{\chi}(z) & = & \int_1^{z} (f'_\diamond(t) + k)\mathrm{d}t \nonumber\\
 & = & f_\diamond(z) - f_\diamond(1) + k (z-1)\:\:.
\end{eqnarray}
So,
\begin{eqnarray}
KL_{\chi}(P\|Q) & \defeq & \expect_{\X\sim
  P}\left[-\log_{\chi}\left(\frac{Q(\X)}{P(\X)}\right)\right]
\nonumber\\
 & = & \expect_{\X\sim
  P}\left[f_\diamond \left(\frac{Q(\X)}{P(\X)}\right)\right] - \expect_{\X\sim
  P}\left[f_\diamond(1) \right] + k \cdot \expect_{\X\sim
  Q}\left[1 \right] - k \cdot \expect_{\X\sim
  P}\left[1 \right]
\nonumber\\
 & = & \expect_{\X\sim
  P}\left[f_\diamond \left(\frac{Q(\X)}{P(\X)}\right)\right] - f_\diamond(1) + k - k 
\nonumber\\
 & = & \expect_{\X\sim
  P}\left[f_\diamond
  \left(\frac{Q(\X)}{P(\X)}\right)\right] \label{eq000}\\
 & = & I_{f_\diamond}(Q\|P) \nonumber\\
 & = & I_f(P\|Q) \:\:,
\end{eqnarray}
as claimed. Eq. (\ref{eq000}) comes from the fact that $f_\diamond(1)
= f(1) = 0$ by assumption. Remark to finish that fixing $k$ as in
eq. (\ref{eqKA}) yields
\begin{eqnarray}
-\log_{\chi}(z) & = & f_\diamond(z) - f_\diamond(1) - (z-1)
f'_\diamond\left(\frac{1}{c}\right)\label{eqLOG1}\:\:.
\end{eqnarray}
If we fix $c = 1$, which is guaranteed to be in $\mathrm{dom} f$, then
we obtain the expression of a Bregman divergence:
\begin{eqnarray}
-\log_{\chi}(z)  & = & D_{f_\diamond}(z\|1)\label{eqLOGCHI1}\:\:.
\end{eqnarray}
In this case, from
eq. (\ref{eqchif}) and our choice of $c$ (and therefore $k$),
\begin{eqnarray}
\chi(z) & = & -\frac{1}{f'_\diamond(z) - f'_\diamond(1)}\nonumber\\
 & = & -\frac{1}{\frac{\mathrm{d} D_{f_\diamond}(z\|1)}{\mathrm{d}z}}\:\:.\label{eqchif2}
\end{eqnarray}
Otherwise, it is possible to tune $c$ in eq. (\ref{eqchif}) or directly
$k$ in ineq. (\ref{constK})
to achieve
additional constraints while keeping the non-negativity of
$\chi$.\\

\noindent We prove point (ii). We have
\begin{eqnarray*}
\expect_{\tilde{{Q}}}[-(\log_\chi({P})-\log_\chi({Q}))]
& = &
\expect_{\tilde{{Q}}}[-(\log_\chi({P})-\log_\chi(\tilde{{Q}}))]
+ \expect_{\tilde{{Q}}}[-(\log_\chi(\tilde{{Q}})-\log_\chi({Q}))]\:\:.
\end{eqnarray*}
Also, 
\begin{eqnarray}
(\log_\chi({P})-\log_\chi({\tilde{{Q}}})) & = & \int_{{{1}}}^P
\frac{1}{\chi(t)} \cdot \mathrm{d}t - \int_1^{\tilde{{Q}}}
\frac{1}{\chi(t)} \cdot \mathrm{d}t\nonumber\\
& = & \int_{\tilde{{Q}}}^P
\frac{1}{\chi(t)} \cdot \mathrm{d}t\nonumber\\
 & = & \int_{1}^{\frac{P}{\tilde{{Q}}}}
\frac{\tilde{{Q}}}{\chi(t \tilde{{Q}})} \cdot \mathrm{d}t\nonumber\\
 & = & \int_{1}^{\frac{P}{\tilde{{Q}}}}
\frac{1}{\chi_{\tilde{{Q}}}(t)} \cdot \mathrm{d}t\nonumber\\
 & = & \log_{\chi_{\tilde{{Q}}}}\left(\frac{P}{\tilde{{Q}}}\right)\:\:,
\end{eqnarray}
with 
\begin{eqnarray}
\chi_{\tilde{{Q}}(\ve{x})}(t) & \defeq & \frac{1}{\tilde{{Q}} (\ve{x})}\cdot \chi
(t\tilde{{Q}}(\ve{x}))\label{defCHITILDE} 
\end{eqnarray}
satisfying $\mathrm{d} \chi_{\tilde{{Q}} (\ve{x})} /
\mathrm{d} t = \chi'
(t \tilde{{Q}} (\ve{x}))$ and so is increasing, plus $\chi_{\tilde{{Q}}}$ is
positive iff $\chi$ is positive since $\tilde{{Q}}(\ve{x})\geq 0$, so $\chi_{\tilde{{Q}}}(t)$
defines a
$\chi$-logarithm, also differentiable. Hence,
\begin{eqnarray}
\expect_{\tilde{{Q}}}[-(\log_\chi({P})-\log_\chi(\tilde{{Q}}))] & = & KL_{\chi_{\tilde{{Q}}}}(\tilde{Q}\|P)\:\:,
\end{eqnarray}
and
\begin{eqnarray}
\expect_{\tilde{{Q}}}[-(\log_\chi({Q}) - \log_\chi(\tilde{{Q}}))] & = & KL_{\chi_{\tilde{{Q}}}}(\tilde{Q}\|Q)\:\:.
\end{eqnarray}
This ends the proof of point (ii).\\

\noindent We prove point (iii). Since $-\log_{\chi}$ is convex, it
follows from Legendre duality,
\begin{eqnarray}
KL_{\chi_{\tilde{{Q}}}}(\tilde{Q}\|P) & = & \sup_{T:
  \mathcal{X}\rightarrow \mathbb{R}} \left\{\expect_{P} [T(\ve{x})]  -
\expect_{\tilde{Q}}
[(-\log_{\chi_{\tilde{Q}}})^\star(T(\ve{x}))]\right\}\nonumber\\
 & = & \sup_{T:
  \mathcal{X}\rightarrow \mathbb{R}} \left\{\expect_{P} [T(\ve{x})]  -
\expect_{\tilde{Q}}
[(-\log_{\chi_{\tilde{Q}}})^\star(T(\ve{x}))]\right\}\nonumber\\
 & = & \sup_{T:
  \mathcal{X}\rightarrow \mathbb{R}} \left\{\expect_{P} [T(\ve{x})]  -
\expect_{\tilde{Q}}
[\log_{\chi^{\bullet}_{\tilde{Q}}} (T(\ve{x}))]\right\} \:\:, \label{varprob}
\end{eqnarray}
with 
\begin{eqnarray}
\chi^{\bullet}(z) & \defeq & \frac{1}{\chi^{-1}\left(\frac{1}{-z}\right)}\:\:.
\end{eqnarray}
The last eq. comes from the following. $-\log_{\chi}$ being
differentiable, its Legendre conjugate has derivative the inverse of the
derivative of $-\log_{\chi}$. Since $(-\log_{\chi})'(z) = -1/\chi(z)$,
its inverse is found to be $((-\log_{\chi})')^{-1}(z) =
\chi^{-1}(-1/z)$, which therefore corresponds to a
$\chi^\bullet$-logarithm with $\chi^\bullet(z) = 1/\chi^{-1}(-1/z)$,
as claimed. Notice that
\begin{eqnarray}
(\log_{\chi^{\bullet}})''(z)  = (1/\chi^\bullet)'(z) & = & \frac{1}{z^2} \cdot \frac{1}{\chi'\left(\chi^{-1}\left(\frac{1}{-z}\right)\right)}\:\:,
\end{eqnarray}
which is non-negative and proves the \textit{convexity} of
$\log_{\chi^{\bullet}}$. To finish-up the proof of point (iii), we
show that the optimal solution $T^*(\ve{x})$ to the variational problem in
eq.(\ref{varprob}) is indeed $T^*(\ve{x}) = -\tilde{Q}(\ve{x}) /
\tilde{P}(\ve{x})$. A pointwise differentiation of eq. (\ref{varprob})
yields that at the optimum, we have 
\begin{eqnarray}
P(\ve{x}) - \tilde{Q}(\ve{x})\cdot \left(
\log_{\chi^\bullet_{\tilde{Q}}}\right)'(T(\ve{x}))) & = & 0\:\:,
\end{eqnarray}
that is, exploiting the fact that $\chi^\bullet(z) = 1/\chi^{-1}(-1/z)$,
\begin{eqnarray}
T^*(\ve{x}) & = & \left(\left(
\log_{\chi^\bullet_{\tilde{Q}}}\right)'\right)^{-1}\left(\frac{P(\ve{x})}{\tilde{Q}(\ve{x})}\right) \nonumber\\
 & = & \left(\frac{1}{\chi^\bullet_{\tilde{Q}}}\right)^{-1}\left(\frac{P(\ve{x})}{\tilde{Q}(\ve{x})}\right) \nonumber\\
 & = &
 -\frac{1}{\chi_{\tilde{Q}} \left(\frac{P(\ve{x})}{\tilde{Q}(\ve{x})}\right)} \label{eqCHIBULLET}\\
 & = &
 -\frac{\tilde{Q}(\ve{x})}{\chi
   \left(\frac{P(\ve{x})}{\tilde{Q}(\ve{x})} \cdot \tilde{Q}(\ve{x})\right)}\nonumber\\
 & = &
 -\frac{\tilde{Q}(\ve{x})}{\chi
   (P(\ve{x}))}\nonumber\\
 & = & - \frac{\tilde{Q}(\ve{x})}{\tilde{P}(\ve{x})}\:\:.\label{eqCHIBUL2}
\end{eqnarray}
In eq. (\ref{eqCHIBULLET}), we have used the fact that
$(1/\chi^\bullet)^{-1}(z) = - 1/\chi(z)$. Notice that because of the
normalization of the escorts, the optimal $T^*$ simplifies to
\begin{eqnarray}
T^*(\ve{x}) & = & - \frac{\chi(Q(\ve{x}))}{\chi(P(\ve{x}))}\:\:.
\end{eqnarray}
