# Supplementary material for: f-GANs in an Information Geometric Nutshell
Source: arXiv:1707.04385 source file (2017-07-14)
Supplement: Supplementary file 2 [file arxiv-gan-appendix.tex]

\section*{\supplement: table of contents}

\noindent Summary of the paper's notations\hrulefill Pg
  \pageref{sec-sum}\\

\noindent \textbf{Supplementary material on proofs and formal results}
\hrulefill Pg \pageref{the_theo}\\ 
\noindent Generalization of Theorem \ref{thmSTAND}\hrulefill Pg
  \pageref{SECGEN}\\
\noindent Proof of Theorem \ref{thDEFEXP1}\hrulefill Pg
  \pageref{proof_thmDEFEXP1}\\
\noindent Proof of Theorem \ref{factorDEEP}\hrulefill Pg
  \pageref{proof_thmfactorDEEP}\\
\noindent Proof of Theorem \ref{thmSUP}\hrulefill Pg
  \pageref{proof_thmSUP}\\
\noindent Proof of Lemma \ref{lemACT}\hrulefill Pg
  \pageref{proof_lemACT}\\
\noindent Proof of Theorem \ref{thmKLQQ}\hrulefill Pg
  \pageref{proof_thmKLQQ}\\
\noindent A more complete picture of admissible activations\hrulefill Pg
  \pageref{sec_admact}\\
\noindent Many modes for GAN architectures\hrulefill Pg
  \pageref{sec_modes}\\
\noindent The two-player vig-$f$-GAN game in the expected utility theory\hrulefill Pg
  \pageref{sec-game}\\

\noindent \textbf{Supplementary material on experiments} \hrulefill
Pg \pageref{exp_expes}\\
\noindent Architectures\hrulefill Pg \pageref{exp_archis}\\
\noindent Experimental setup for varying the activation function in the
generator\hrulefill Pg
  \pageref{exp_gen}\\
\noindent Visual results\hrulefill Pg
  \pageref{exp_mnist}\\
$\hookrightarrow$ MNIST results for GAN$\_$DCGAN at varying $\mu$ ($\mu=1$ is ReLU)\hrulefill Pg
  \pageref{tab:expes_visu_mnist_gan_dcgan}\\
$\hookrightarrow$ MNIST results for WGAN$\_$DCGAN at varying $\mu$ ($\mu=1$ is ReLU)\hrulefill Pg
  \pageref{tab:expes_visu_mnist_wgan_dcgan}\\
$\hookrightarrow$ MNIST results for WGAN$\_$MLP at varying $\mu$ ($\mu=1$ is ReLU)\hrulefill Pg
  \pageref{tab:expes_visu_mnist_wgan_mlp}\\
$\hookrightarrow$ MNIST results for GAN$\_$MLP at varying $\mu$ ($\mu=1$ is ReLU)\hrulefill Pg
  \pageref{tab:expes_visu_mnist_gan_mlp}\\
$\hookrightarrow$ LSUN results for GAN$\_$DCGAN at varying $\mu$ ($\mu=1$ is ReLU)\hrulefill Pg
  \pageref{tab:expes_visu_lsun}

\newpage

\section{Summary of the paper's notations}\label{sec-sum}

\begin{figure}[t]
\begin{center}
\begin{tabular}{c}
\includegraphics[trim=30bp 270bp 420bp
20bp,clip,width=0.80\columnwidth]{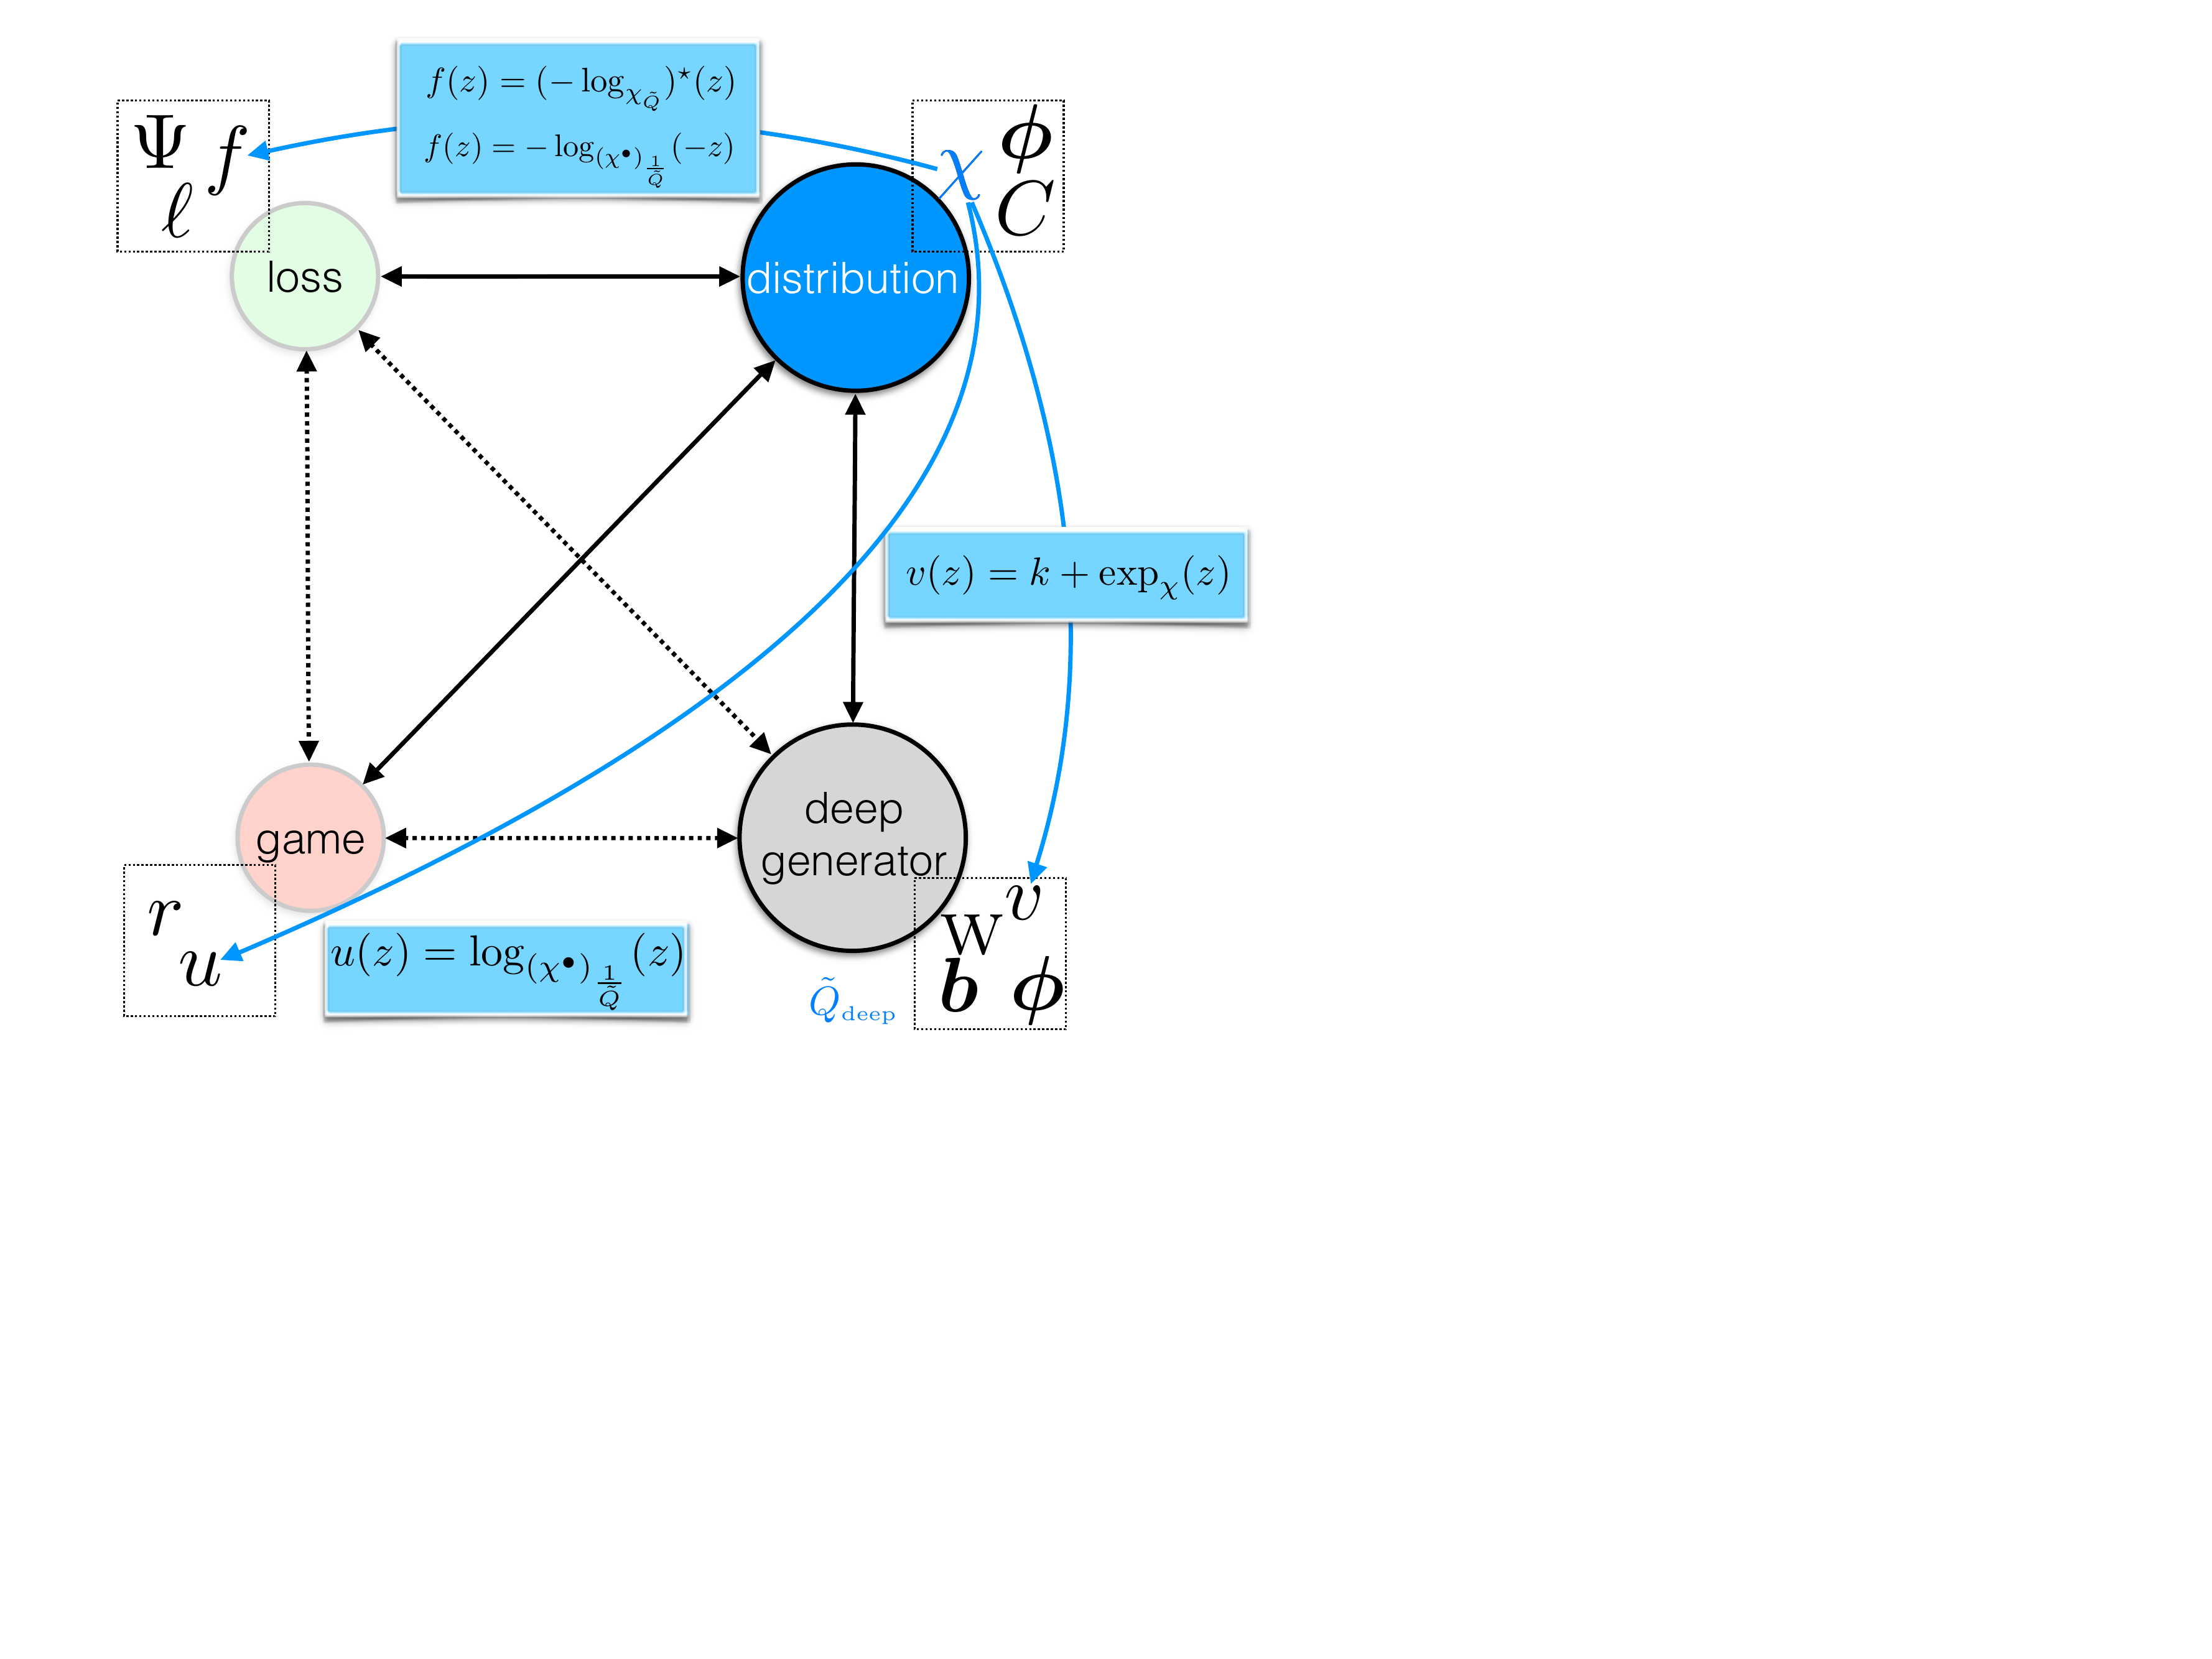} 
\end{tabular} 
\end{center}
\caption{Summary of the main notations with respect to the GAN
  game, according to the four main parameters of the game (loss,
  density, game, model = deep generator). Plain (black / blue) arcs
  denote formal relationships that we show. 
The density of a deep generator
  decomposes in three parts, one which depends on the simple input
  density, one which depends on the very last layer and one which
  incorporates all the deep architecture components,
  $\tilde{Q}_{\mbox{\tiny{deep}}}$ (Theorem
  \ref{factorDEEP}). $\tilde{Q}_{\mbox{\tiny{deep}}}$ (shown) precisely
  factors escorts numbers of deformed exponential families.}
\label{f-summa}
\end{figure}

Figure \ref{f-summa} summarizes the main notations with respect to our contributions on
the four components of the GAN quadrangle: loss, density, game and
models ( = deep generator). Blue arcs identify some
  key paramaters as a function of the signature of the deformed
  exponential family, $\chi$, to match several quantities of interest: 
\begin{itemize}
\item the arc $\chi \rightarrow
  f$ identifies the $f$ from $\chi$ which allows to prove the identity
  between vig-$f$-GAN and the $f$-GAN identity in \cite{nctFG}
  (Theorem \ref{thDEFEXP1});
\item the arc $\chi \rightarrow v$ identifies the activation function
  $v$ from $\chi$
  for which the inner deep part of the generator in Theorem
  \ref{factorDEEP};
\item the arc $\chi \rightarrow u$ identifies the utility function of
  the discriminator / decision maker such that the decision maker's
  utility $U(\mathcal{Q})$ maximization (eq. (\ref{defEU})) matches
  vig-$f$-GAN (Lemma \ref{lemGAME}).
\end{itemize}
Name are as follows:
\begin{itemize}
\item [\textsc{loss}] $f$ = generator of the $f$-divergence; $\ell$ =
  loss function for the supervised game; $\Psi$ = link function for
  the supervised loss;
 \item [\textsc{density}] $\chi$ = signature of the deformed
   exponential family; $\ve{\phi}$ = sufficient statistics; $C$ =
   cumulant;
\item [\textsc{game}] $u$ = utility function; $r$ = Arrow-Pratt
  coefficient of risk
  aversion;
\item [\textsc{model}] $\matrice{w}$ = inner layer matrices; $\ve{b}$
  = inner layers bias vectors; $v$ = inner layers activation function;
  $\ve{\phi}$ = inner layers vectors;
\end{itemize}

\newpage

\section*{Supplementary material on proofs and formal results}\label{the_theo}

\section{Generalization of Theorem \ref{thmSTAND}}\label{SECGEN}
\input{arxiv-gan-proof-thmSTAND}

\section{Proof of Theorem \ref{thDEFEXP1}}\label{proof_thmDEFEXP1}

Without loss of generality we can assume that $\sup \mathbb{I}_{P,Q} <
+\infty$. Otherwise, when $\sup \mathbb{I}_{P,Q} = + \infty$,
requesting $\sup \xi(\mathbb{I}_{P,Q}) = +\infty$ ($\forall \xi \in \partial
f$) implies, because $f$
is convex continuous, that $\lim_{\sup
  \mathbb{I}_{P,Q}}f(z) = +\infty$, and so the constraint $I_f(P\|Q) <
+\infty$ essentially enforces zero measure over all infinite density ratios.

We make use of \cite[Proposition 1.6.1]{npCF}, now with a
subdifferential which is not Riemann integrable in $M \defeq \sup
\mathbb{I}_{P,Q}$. Notice that we can assume without loss of
generality that $M > 1$ since otherwise, since it is convex and
continuous, $f$ would not be defined for $z> 1$ and $I_f(P\|Q)$
would essentially be infinite unless $Q \geq P$ almost everywhere
(\textit{i.e.} $P$ dominates $Q$ only on sets of zero measure).\\

For any constants
$t^* < M, \epsilon$ such that $\xi(t^*) < +\infty$, let
\begin{eqnarray}
g_{t^*,\epsilon}(z) & \defeq & \int_{1}^{z}
(-\xi(t)+\xi(t^*)+\epsilon)\mathrm{d}t\:\:, 
\end{eqnarray}
where $z \in \mathbb{R}_+$ is any real such that the integral in
$g_{t^*,\epsilon}$ is not improper
(therefore, $z< M$). Let
\begin{eqnarray}
\chi_{t^*,\epsilon}(t) & = & \left\{
\begin{array}{rcl}
\frac{1}{-\xi(t) +\xi(t^*)+\epsilon} & \mbox{ if } & t < t^*\:\:,\\
\frac{1}{\epsilon} & \mbox{ if } & t \geq t^*
\end{array}
\right.\:\:,
\end{eqnarray}
which, if $\epsilon > 0$, is non negative and also increasing
since $\xi $ is increasing. Consider any fixed $z^* \in \mathbb{I}_{P,Q}
\cap (1,\infty)$ with $0<\xi(z^*) < \infty$ and let $t^* \defeq \sup
\{z : \xi(z) \leq \xi(z^*)\}$. We have:
\begin{eqnarray}
g_{t^*,\epsilon}(z) & = & \int_{1}^{z}
(-\xi(t)+\xi(t^*)+\epsilon)\mathrm{d}t\nonumber\\
& = & \int_{1}^{z}
\frac{1}{\chi_{t^*,\epsilon}(t)} \mathrm{d}t + 1_{[z \geq t^*]} \cdot \int_{t^*}^{z}
(-\xi(t)+ \xi(t^*))\mathrm{d}t\nonumber\\
& =  & \int_{1}^{z}
\frac{1}{\chi_{t^*,\epsilon}(t)} \mathrm{d}t  -
1_{[z \geq t^*]} \cdot \int_{t^*}^{z}
(\xi(t)- \xi(t^*))\mathrm{d}t\nonumber\\
 & = & \int_{1}^{z}
\frac{1}{\chi_{t^*,\epsilon}(t)} \mathrm{d}t  -
1_{[z\geq t^*]} \cdot D_{f,
  \xi}\left(\left. z\right\| t^*\right) \label{inv3}\:\:.
\end{eqnarray}
The last identity comes from \cite[Proposition 1.6.1]{npCF} and the
fact that $\xi(t)- \xi(t^*)$ belongs to the subdifferential of the
Bregman divergence whose generator is $f$ \cite{frCF}. We obtain:
\begin{eqnarray}
\lefteqn{\expect_{\X\sim
  Q}\left[f
  \left(\frac{P(\X)}{Q(\X)}\right)\right]}\nonumber\\
 & = & \expect_{\X\sim
  Q}\left[f_{\xi(t^*)+\epsilon}
  \left(\frac{P(\X)}{Q(\X)}\right)\right]\label{cons11}\\
 & = & \expect_{\X\sim
  Q}\left[\lim_{\rho \rightarrow \frac{P(\X)}{Q(\X)}} -\int_{1}^{\rho}
(-\xi(t)+\xi(t^*)+\epsilon) \mathrm{d}t\right]\label{cons12}\\
 & = & \expect_{\X\sim
  Q}\left[\lim_{\rho \rightarrow \frac{P(\X)}{Q(\X)}} -g_{t^*,\epsilon}(\rho)\right]\nonumber\\
 & = & \expect_{\X\sim
  Q}\left[\lim_{\rho \rightarrow \frac{P(\X)}{Q(\X)}}
  \left\{-\int_{1}^{\rho}
\frac{1}{\chi_{t^*,\epsilon}(t)} \mathrm{d}t +
1_{\left[\rho\geq t^*\right]} \cdot D_{f,
  \xi}\left(\left. \rho \right\| t^*\right) \right\}\right]\label{cons13}\\
 & = & \expect_{\X\sim
  Q}\left[-\lim_{\rho \rightarrow \frac{P(\X)}{Q(\X)}}
  \int_{1}^{\rho}
\frac{1}{\chi_{t^*,\epsilon}(t)} \mathrm{d}t\right] + \underbrace{\expect_{\X\sim
  Q}\left[\lim_{\rho \rightarrow \frac{P(\X)}{Q(\X)}}
1_{\left[\rho\geq t^*\right]} \cdot D_{f,
  \xi}\left(\left. \rho \right\| t^*\right) \right]}_{\defeq R(t^*)}\label{cons15}\\
 & = & \expect_{\X\sim
  Q}\left[-\log_{\chi_{t^*,\epsilon}}\left(\frac{P(\X)}{
      Q(\X)}\right)\right] + R(t^*)\label{cons16}\\
 & = & KL_{\chi_{t^*,\epsilon}}(Q\|P) + R(t^*)\label{cons17}\:\:.
\end{eqnarray}
Eq. (\ref{cons11}) follows from Eq. (\ref{inv1}).
Eq. (\ref{cons12}) follows from Eq. (\ref{inv2}).
Eq. (\ref{cons13}) follows from Eq. (\ref{inv3}). We can split the
limits in eq. (\ref{cons15}) because each term in the expectation of
$R(t^*)$ is finite. To see it, since $I_f(P\|Q) < \infty$ and $\sup
\xi (\mathbb{I}_{P,Q}) = +\infty$, we can assume that $f(M) <
+\infty$. Since $\xi(t^*) \geq
0$, then
\begin{eqnarray}
\rho \geq t^* & \Rightarrow & D_{f,
  \xi}\left(\left. \rho \right\| t^*\right) \leq f(M) - f(t^*) \:\:,
\end{eqnarray}
which is indeed finite. It then comes 
\begin{eqnarray}
\expect_{\X\sim
  Q}\left[\lim_{\rho \rightarrow \frac{P(\X)}{Q(\X)}}
1_{\left[\rho\geq t^*\right]} \cdot D_{f,
  \xi}\left(\left. \rho \right\| t^*\right) \right] & = & \expect_{\X\sim
  Q}\left[
1_{\left[\frac{P(\X)}{Q(\X)}\geq t^*\right]} \cdot D_{f,
  \xi}\left(\left. \frac{P(\X)}{Q(\X)} \right\| t^*\right)
\right]\nonumber\\
 & \leq & \expect_{\X\sim
  Q}\left[D_{f,
  \xi}(M\|t^*)
\right] \nonumber\\
 & \leq & f(M) - f(t^*)\:\:.
\end{eqnarray}
Since $f$ is continuous, we get the upperbound on $I_f(P\|Q)$ by choosing $t^*<M$ as
close as desired to $M$. We get the lowerbound by remarking that
$R(t^*) \geq 0$ (a Bregman divergence cannot be negative).

\newpage

\begin{theorem}
Letting
$P\defeq P_{\chi, C}$ and $Q \defeq Q_{\chi, C}$ for short, the following holds:
\begin{eqnarray}
\expect_{\X\sim \tilde{Q}}[\log_\chi(Q(\X)) - \log_\chi(P(\X))] & = &
KL_{\chi_{\tilde{{Q}}}}(\tilde{Q}\|P) - J(Q)\:\:,
\end{eqnarray} 
with $J(Q) \defeq
KL_{\chi_{\tilde{{Q}}}}(\tilde{Q}\|Q)$ and $\chi_{\tilde{Q}(\ve{x})}(t) \defeq (1/\tilde{Q}(\ve{x}))\cdot \chi
(t \tilde{Q}(\ve{x}))$.
\end{theorem}
The normalization $Z$ for the escort of $Q$ being
finite, it implies the finiteness of $\tilde{Q}$ almost everywhere

We have
\begin{eqnarray*}
\expect_{\tilde{{Q}}}[-(\log_\chi({P})-\log_\chi({Q}))]
& = &
\expect_{\tilde{{Q}}}[-(\log_\chi({P})-\log_\chi(\tilde{{Q}}))]
+ \expect_{\tilde{{Q}}}[-(\log_\chi(\tilde{{Q}})-\log_\chi({Q}))]\:\:.
\end{eqnarray*}
Also, 
\begin{eqnarray}
(\log_\chi({P})-\log_\chi({\tilde{{Q}}})) & = & \int_{{{1}}}^P
\frac{1}{\chi(t)} \cdot \mathrm{d}t - \int_1^{\tilde{{Q}}}
\frac{1}{\chi(t)} \cdot \mathrm{d}t\nonumber\\
& = & \int_{\tilde{{Q}}}^P
\frac{1}{\chi(t)} \cdot \mathrm{d}t\nonumber\\
 & = & \int_{1}^{\frac{P}{\tilde{{Q}}}}
\frac{\tilde{{Q}}}{\chi(t \tilde{{Q}})} \cdot \mathrm{d}t\nonumber\\
 & = & \int_{1}^{\frac{P}{\tilde{{Q}}}}
\frac{1}{\chi_{\tilde{{Q}}}(t)} \cdot \mathrm{d}t\nonumber\\
 & = & \log_{\chi_{\tilde{{Q}}}}\left(\frac{P}{\tilde{{Q}}}\right)\:\:,
\end{eqnarray}
with 
\begin{eqnarray}
\chi_{\tilde{{Q}}(\ve{x})}(t) & \defeq & \frac{1}{\tilde{{Q}} (\ve{x})}\cdot \chi
(t\tilde{{Q}}(\ve{x}))\label{defCHITILDE} 
\end{eqnarray}
satisfying $\mathrm{d} \chi_{\tilde{{Q}} (\ve{x})} /
\mathrm{d} t = \chi'
(t \tilde{{Q}} (\ve{x}))$ and so is increasing, plus $\chi_{\tilde{{Q}}}$ is
positive iff $\chi$ is positive since $\tilde{{Q}}(\ve{x})\geq 0$, so $\chi_{\tilde{{Q}}}(t)$
defines a
$\chi$-logarithm, also differentiable. Hence,
\begin{eqnarray}
\expect_{\tilde{{Q}}}[-(\log_\chi({P})-\log_\chi(\tilde{{Q}}))] & = & KL_{\chi_{\tilde{{Q}}}}(\tilde{Q}\|P)\:\:,
\end{eqnarray}
and
\begin{eqnarray}
\expect_{\tilde{{Q}}}[-(\log_\chi({Q}) - \log_\chi(\tilde{{Q}}))] & = & KL_{\chi_{\tilde{{Q}}}}(\tilde{Q}\|Q)\:\:.
\end{eqnarray}
This ends the proof of point (ii).\\

\newpage

\noindent We prove point (i). We first remark that we have $(-\log_{\chi})'' = \chi' / \chi^2 \geq 0$ and so $-\log_{\chi}$ is convex and $KL_{\chi}(P\|Q)$ is an
$f$-divergence with $f$ twice differentiable. We also notice that
$\mathrm{dom}(-\log_{\chi}) \supseteq \mathbb{R}_+$.
To show the equivalence, we extract $\chi$ from any
twice differentiable $f$-divergence and show that for this couple $(f,
\chi)$,
$KL_{\chi}(P\|Q) = I_f(P\|Q), \forall P, Q$. Let $f_\diamond(z)
\defeq z \cdot f(1/z)$ denote the Csisz\'ar dual of $f$, which is
also convex (indeed, $f''_\diamond(z) = (1/z^2)\cdot f''(z)$) and
satisfies $I_f(P\|Q) = I_{f_\diamond}(Q\|P)$. Hence, we want to prove
\begin{eqnarray}
\expect_{\X\sim P}\left[-\log_{\chi}\left(\frac{Q(\X)}{P(\X)}\right)\right] & = & \expect_{\X\sim P}
\left[f_\diamond \left(\frac{Q(\X)}{P(\X)}\right)\right]\:\:, \forall
P, Q\:\:.
\end{eqnarray}
We want 
\begin{eqnarray}
\frac{\chi'}{\chi^2} & = & f''_\diamond\:\:,
\end{eqnarray}
whose solution is easily found to be solution to the following
differential equation: $\mathrm{d}\left(-1/\chi(z)\right) = f''_\diamond(z)
\mathrm{d} z$, that is, $-1/\chi(z) = f'_\diamond(z) + k$ for any constant $k$
and therefore
\begin{eqnarray}
\chi(z) & = & -\frac{1}{f'_\diamond(z) + k}\:\:,\label{eqchif}
\end{eqnarray}
Clearly, $\chi$ is increasing since $f_\diamond$ is convex and
\begin{eqnarray}
\chi'(z) & = & \frac{f''_\diamond(z)}{(f'_\diamond(z) + k)^2}\:\:.
\end{eqnarray}
 We now
constrain the choice of $k$ to the fact that we also want $\chi(z)\geq
0$, that is, we want $k$ such that 
\begin{eqnarray}
f'_\diamond(z) & \leq & -k\:\:, \forall z\in \mathbb{R}_+\:\:.\label{constK}
\end{eqnarray}
To prove that this is indeed possible, we first remark
that for any constant $k_2\geq 0$, 
\begin{eqnarray}
f'(t) & \leq & f'(t) + t f''(t) + k_2 \:\:,\forall t\geq 0\:\:.\label{eqCONV1}
\end{eqnarray}
This is indeed obvious since $f$ is convex, and it brings after
integration between any constant $c \in \mathrm{dom} f'$ and $z$,
$f(z) - f(c) \leq z f'(z) - c f'(c) + k_2 (z-c)$, which
brings after the change of variable $z\mapsto 1/z$ and reordering:
\begin{eqnarray}
\underbrace{f\left(\frac{1}{z}\right) - \frac{1}{z} \cdot
f'\left(\frac{1}{z}\right)}_{= f'_\diamond(z)} & \leq & \frac{k_2}{z} + f(c) - cf'(c) - ck_2 \:\:,
\end{eqnarray}
so we get that we can pick $k_2=0$ which, to guarantee ineq. (\ref{constK}), yields \textit{e.g.} the choice
\begin{eqnarray}
k & = & -(f(c) - cf'(c)) = - f'_\diamond(1/c)\:\:, \label{eqKA}
\end{eqnarray}
with $c \in \mathrm{dom} f'$. For the
expression of $\chi$ in (\ref{eqchif}), we obtain 
\begin{eqnarray}
-\log_{\chi}(z) & = & \int_1^{z} (f'_\diamond(t) + k)\mathrm{d}t \nonumber\\
 & = & f_\diamond(z) - f_\diamond(1) + k (z-1)\:\:.
\end{eqnarray}
So,
\begin{eqnarray}
KL_{\chi}(P\|Q) & \defeq & \expect_{\X\sim
  P}\left[-\log_{\chi}\left(\frac{Q(\X)}{P(\X)}\right)\right]
\nonumber\\
 & = & \expect_{\X\sim
  P}\left[f_\diamond \left(\frac{Q(\X)}{P(\X)}\right)\right] - \expect_{\X\sim
  P}\left[f_\diamond(1) \right] + k \cdot \expect_{\X\sim
  Q}\left[1 \right] - k \cdot \expect_{\X\sim
  P}\left[1 \right]
\nonumber\\
 & = & \expect_{\X\sim
  P}\left[f_\diamond \left(\frac{Q(\X)}{P(\X)}\right)\right] - f_\diamond(1) + k - k 
\nonumber\\
 & = & \expect_{\X\sim
  P}\left[f_\diamond
  \left(\frac{Q(\X)}{P(\X)}\right)\right] \label{eq000}\\
 & = & I_{f_\diamond}(Q\|P) \nonumber\\
 & = & I_f(P\|Q) \:\:,
\end{eqnarray}
as claimed. Eq. (\ref{eq000}) comes from the fact that $f_\diamond(1)
= f(1) = 0$ by assumption. Remark to finish that fixing $k$ as in
eq. (\ref{eqKA}) yields
\begin{eqnarray}
-\log_{\chi}(z) & = & f_\diamond(z) - f_\diamond(1) - (z-1)
f'_\diamond\left(\frac{1}{c}\right)\label{eqLOG1}\:\:.
\end{eqnarray}
If we fix $c = 1$, which is guaranteed to be in $\mathrm{dom} f$, then
we obtain the expression of a Bregman divergence:
\begin{eqnarray}
-\log_{\chi}(z)  & = & D_{f_\diamond}(z\|1)\label{eqLOGCHI1}\:\:.
\end{eqnarray}
In this case, from
eq. (\ref{eqchif}) and our choice of $c$ (and therefore $k$),
\begin{eqnarray}
\chi(z) & = & -\frac{1}{f'_\diamond(z) - f'_\diamond(1)}\nonumber\\
 & = & -\frac{1}{\frac{\mathrm{d} D_{f_\diamond}(z\|1)}{\mathrm{d}z}}\:\:.\label{eqchif2}
\end{eqnarray}
Otherwise, it is possible to tune $c$ in eq. (\ref{eqchif}) or directly
$k$ in ineq. (\ref{constK})
to achieve
additional constraints while keeping the non-negativity of
$\chi$.\\

\noindent We prove point (ii). We have
\begin{eqnarray*}
\expect_{\tilde{{Q}}}[-(\log_\chi({P})-\log_\chi({Q}))]
& = &
\expect_{\tilde{{Q}}}[-(\log_\chi({P})-\log_\chi(\tilde{{Q}}))]
+ \expect_{\tilde{{Q}}}[-(\log_\chi(\tilde{{Q}})-\log_\chi({Q}))]\:\:.
\end{eqnarray*}
Also, 
\begin{eqnarray}
(\log_\chi({P})-\log_\chi({\tilde{{Q}}})) & = & \int_{{{1}}}^P
\frac{1}{\chi(t)} \cdot \mathrm{d}t - \int_1^{\tilde{{Q}}}
\frac{1}{\chi(t)} \cdot \mathrm{d}t\nonumber\\
& = & \int_{\tilde{{Q}}}^P
\frac{1}{\chi(t)} \cdot \mathrm{d}t\nonumber\\
 & = & \int_{1}^{\frac{P}{\tilde{{Q}}}}
\frac{\tilde{{Q}}}{\chi(t \tilde{{Q}})} \cdot \mathrm{d}t\nonumber\\
 & = & \int_{1}^{\frac{P}{\tilde{{Q}}}}
\frac{1}{\chi_{\tilde{{Q}}}(t)} \cdot \mathrm{d}t\nonumber\\
 & = & \log_{\chi_{\tilde{{Q}}}}\left(\frac{P}{\tilde{{Q}}}\right)\:\:,
\end{eqnarray}
with 
\begin{eqnarray}
\chi_{\tilde{{Q}}(\ve{x})}(t) & \defeq & \frac{1}{\tilde{{Q}} (\ve{x})}\cdot \chi
(t\tilde{{Q}}(\ve{x}))\label{defCHITILDE} 
\end{eqnarray}
satisfying $\mathrm{d} \chi_{\tilde{{Q}} (\ve{x})} /
\mathrm{d} t = \chi'
(t \tilde{{Q}} (\ve{x}))$ and so is increasing, plus $\chi_{\tilde{{Q}}}$ is
positive iff $\chi$ is positive since $\tilde{{Q}}(\ve{x})\geq 0$, so $\chi_{\tilde{{Q}}}(t)$
defines a
$\chi$-logarithm, also differentiable. Hence,
\begin{eqnarray}
\expect_{\tilde{{Q}}}[-(\log_\chi({P})-\log_\chi(\tilde{{Q}}))] & = & KL_{\chi_{\tilde{{Q}}}}(\tilde{Q}\|P)\:\:,
\end{eqnarray}
and
\begin{eqnarray}
\expect_{\tilde{{Q}}}[-(\log_\chi({Q}) - \log_\chi(\tilde{{Q}}))] & = & KL_{\chi_{\tilde{{Q}}}}(\tilde{Q}\|Q)\:\:.
\end{eqnarray}
This ends the proof of point (ii).\\

\noindent We prove point (iii). Since $-\log_{\chi}$ is convex, it
follows from Legendre duality,
\begin{eqnarray}
KL_{\chi_{\tilde{{Q}}}}(\tilde{Q}\|P) & = & \sup_{T:
  \mathcal{X}\rightarrow \mathbb{R}} \left\{\expect_{P} [T(\ve{x})]  -
\expect_{\tilde{Q}}
[(-\log_{\chi_{\tilde{Q}}})^\star(T(\ve{x}))]\right\}\nonumber\\
 & = & \sup_{T:
  \mathcal{X}\rightarrow \mathbb{R}} \left\{\expect_{P} [T(\ve{x})]  -
\expect_{\tilde{Q}}
[(-\log_{\chi_{\tilde{Q}}})^\star(T(\ve{x}))]\right\}\nonumber\\
 & = & \sup_{T:
  \mathcal{X}\rightarrow \mathbb{R}} \left\{\expect_{P} [T(\ve{x})]  -
\expect_{\tilde{Q}}
[\log_{\chi^{\bullet}_{\tilde{Q}}} (T(\ve{x}))]\right\} \:\:, \label{varprob}
\end{eqnarray}
with 
\begin{eqnarray}
\chi^{\bullet}(z) & \defeq & \frac{1}{\chi^{-1}\left(\frac{1}{-z}\right)}\:\:.
\end{eqnarray}
The last eq. comes from the following. $-\log_{\chi}$ being
differentiable, its Legendre conjugate has derivative the inverse of the
derivative of $-\log_{\chi}$. Since $(-\log_{\chi})'(z) = -1/\chi(z)$,
its inverse is found to be $((-\log_{\chi})')^{-1}(z) =
\chi^{-1}(-1/z)$, which therefore corresponds to a
$\chi^\bullet$-logarithm with $\chi^\bullet(z) = 1/\chi^{-1}(-1/z)$,
as claimed. Notice that
\begin{eqnarray}
(\log_{\chi^{\bullet}})''(z)  = (1/\chi^\bullet)'(z) & = & \frac{1}{z^2} \cdot \frac{1}{\chi'\left(\chi^{-1}\left(\frac{1}{-z}\right)\right)}\:\:,
\end{eqnarray}
which is non-negative and proves the \textit{convexity} of
$\log_{\chi^{\bullet}}$. To finish-up the proof of point (iii), we
show that the optimal solution $T^*(\ve{x})$ to the variational problem in
eq.(\ref{varprob}) is indeed $T^*(\ve{x}) = -\tilde{Q}(\ve{x}) /
\tilde{P}(\ve{x})$. A pointwise differentiation of eq. (\ref{varprob})
yields that at the optimum, we have 
\begin{eqnarray}
P(\ve{x}) - \tilde{Q}(\ve{x})\cdot \left(
\log_{\chi^\bullet_{\tilde{Q}}}\right)'(T(\ve{x}))) & = & 0\:\:,
\end{eqnarray}
that is, exploiting the fact that $\chi^\bullet(z) = 1/\chi^{-1}(-1/z)$,
\begin{eqnarray}
T^*(\ve{x}) & = & \left(\left(
\log_{\chi^\bullet_{\tilde{Q}}}\right)'\right)^{-1}\left(\frac{P(\ve{x})}{\tilde{Q}(\ve{x})}\right) \nonumber\\
 & = & \left(\frac{1}{\chi^\bullet_{\tilde{Q}}}\right)^{-1}\left(\frac{P(\ve{x})}{\tilde{Q}(\ve{x})}\right) \nonumber\\
 & = &
 -\frac{1}{\chi_{\tilde{Q}} \left(\frac{P(\ve{x})}{\tilde{Q}(\ve{x})}\right)} \label{eqCHIBULLET}\\
 & = &
 -\frac{\tilde{Q}(\ve{x})}{\chi
   \left(\frac{P(\ve{x})}{\tilde{Q}(\ve{x})} \cdot \tilde{Q}(\ve{x})\right)}\nonumber\\
 & = &
 -\frac{\tilde{Q}(\ve{x})}{\chi
   (P(\ve{x}))}\nonumber\\
 & = & - \frac{\tilde{Q}(\ve{x})}{\tilde{P}(\ve{x})}\:\:.\label{eqCHIBUL2}
\end{eqnarray}
In eq. (\ref{eqCHIBULLET}), we have used the fact that
$(1/\chi^\bullet)^{-1}(z) = - 1/\chi(z)$. Notice that because of the
normalization of the escorts, the optimal $T^*$ simplifies to
\begin{eqnarray}
T^*(\ve{x}) & = & - \frac{\chi(Q(\ve{x}))}{\chi(P(\ve{x}))}\:\:.
\end{eqnarray}
